# Supplementary material for: ALMA-IMF. VII. First release of the full spectral line cubes: Core kinematics traced by DCN J=(3-2)
Source: arXiv:2306.14710 source file (2023-06-26)
Supplement: Supplementary file 23 [file corefits_t.tex]

\begin{figure*}
    \centering
\includegraphics[width=0.24\textwidth]{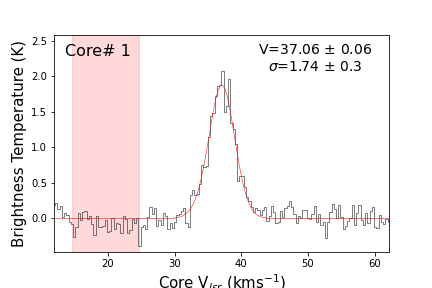}
\includegraphics[width=0.24\textwidth]{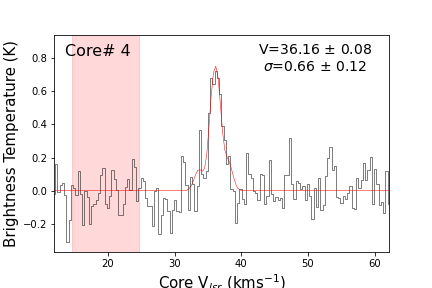}
\includegraphics[width=0.24\textwidth]{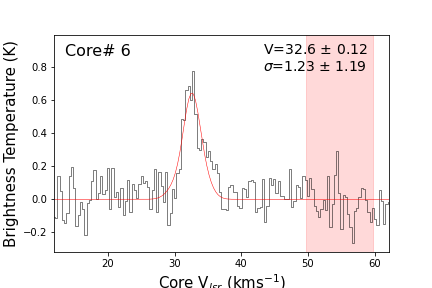}
\includegraphics[width=0.24\textwidth]{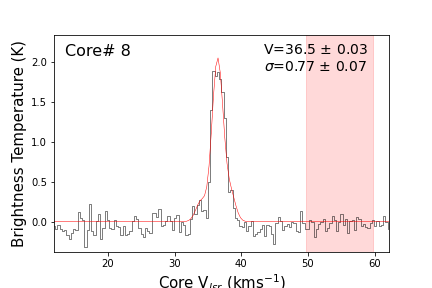}
\includegraphics[width=0.24\textwidth]{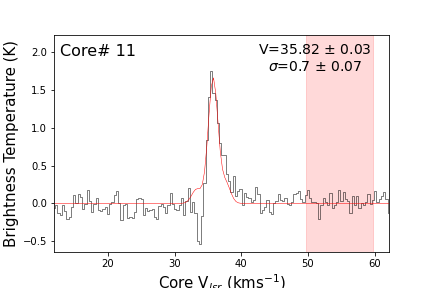}
\includegraphics[width=0.24\textwidth]{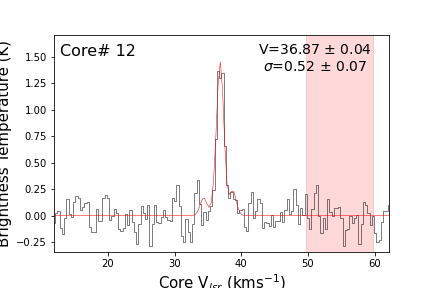}
\includegraphics[width=0.24\textwidth]{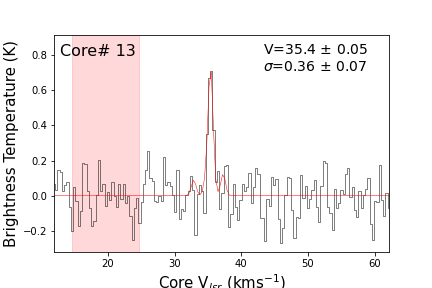}
\includegraphics[width=0.24\textwidth]{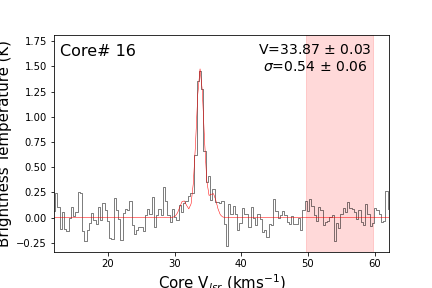}
\includegraphics[width=0.24\textwidth]{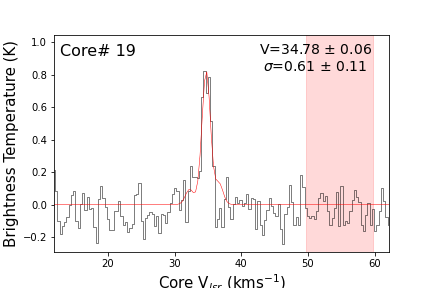}
\includegraphics[width=0.24\textwidth]{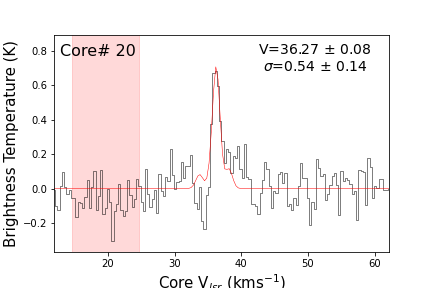}
\includegraphics[width=0.24\textwidth]{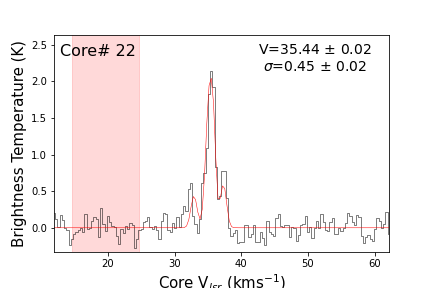}
\includegraphics[width=0.24\textwidth]{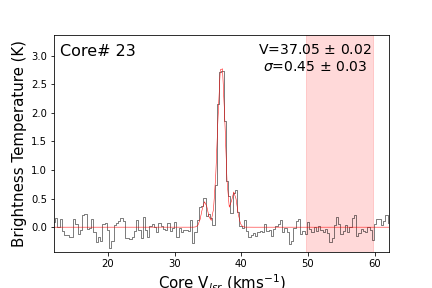}
\includegraphics[width=0.24\textwidth]{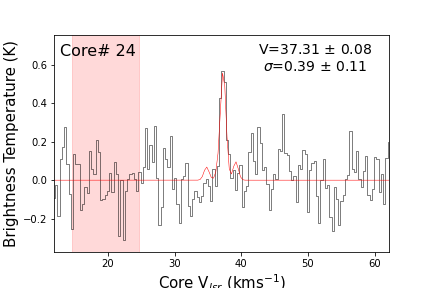}
\includegraphics[width=0.24\textwidth]{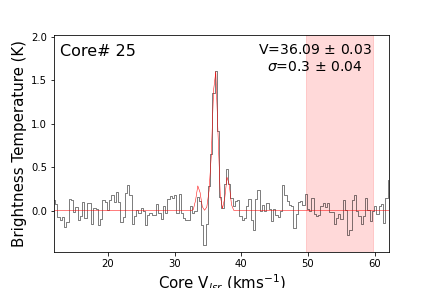}
\includegraphics[width=0.24\textwidth]{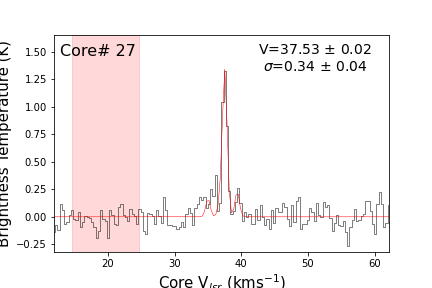}
\includegraphics[width=0.24\textwidth]{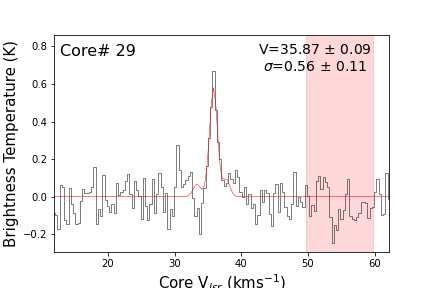}
\includegraphics[width=0.24\textwidth]{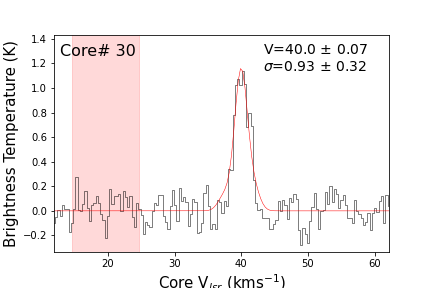}
\includegraphics[width=0.24\textwidth]{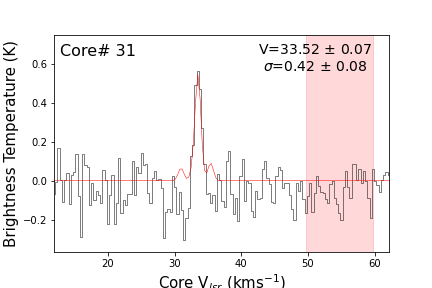}
\includegraphics[width=0.24\textwidth]{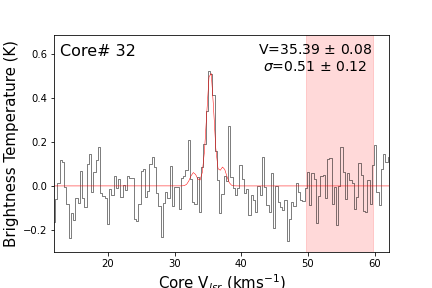}
\includegraphics[width=0.24\textwidth]{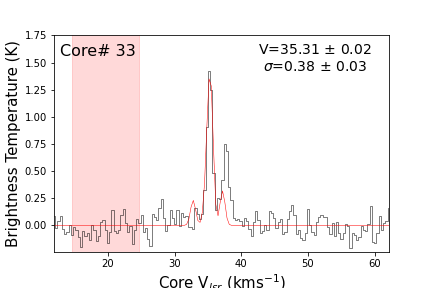}
\includegraphics[width=0.24\textwidth]{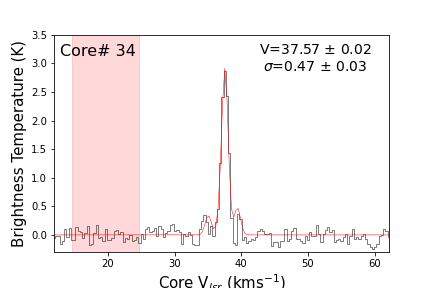}
\includegraphics[width=0.24\textwidth]{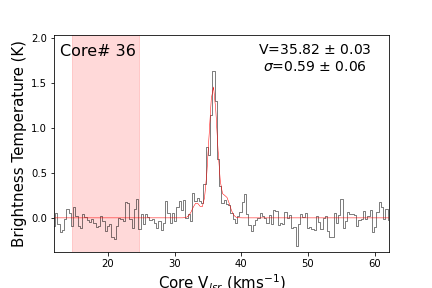}
\includegraphics[width=0.24\textwidth]{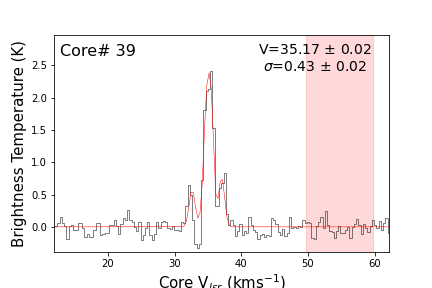}
\includegraphics[width=0.24\textwidth]{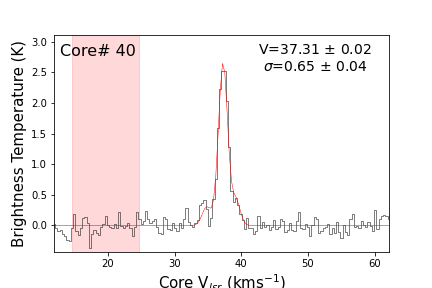}
\includegraphics[width=0.24\textwidth]{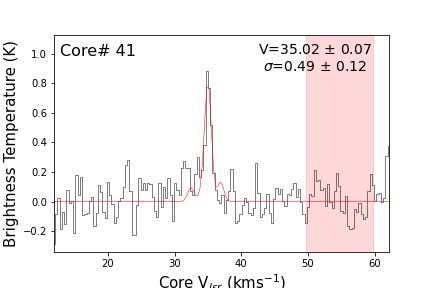}
\includegraphics[width=0.24\textwidth]{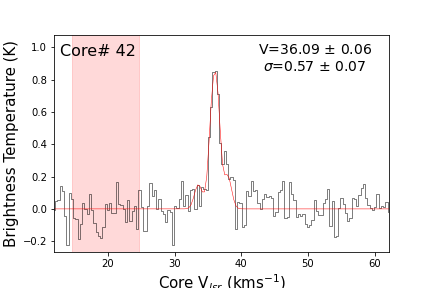}
\includegraphics[width=0.24\textwidth]{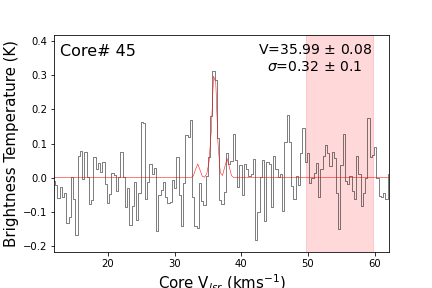}
\includegraphics[width=0.24\textwidth]{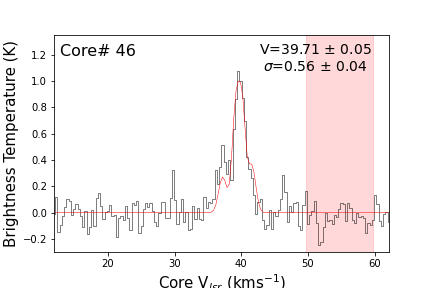}

\caption{Single-type spectra from the background subtracted DCN emission extracted towards the cores in the evolved protocluster G012.80. These spectra are defined as a Single component and used in the analysis. See \cref{tabappendix:coretables_g012} for the line fit parameters for each core.\label{figspectra:dcnspectra_split_G012_s}}
\end{figure*}

\begin{figure*}\ContinuedFloat
    \centering
\includegraphics[width=0.24\textwidth]{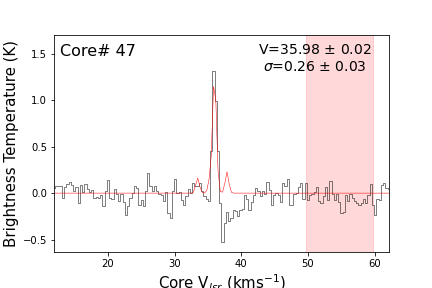}
\includegraphics[width=0.24\textwidth]{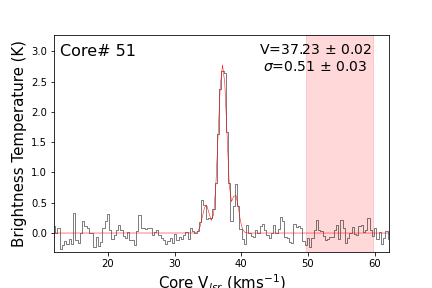}
\includegraphics[width=0.24\textwidth]{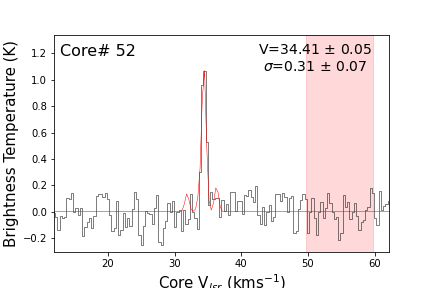}
\includegraphics[width=0.24\textwidth]{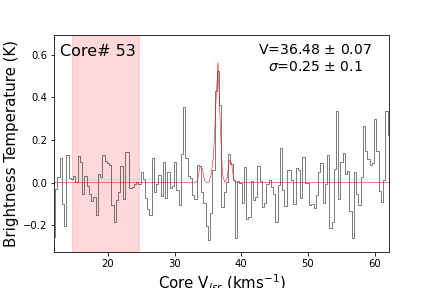}

\includegraphics[width=0.24\textwidth]{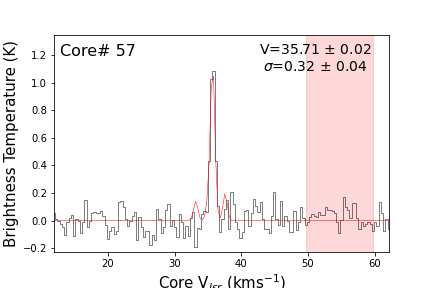}
\includegraphics[width=0.24\textwidth]{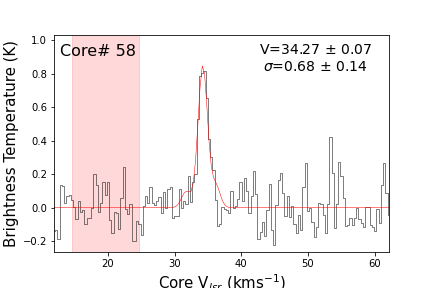}
\includegraphics[width=0.24\textwidth]{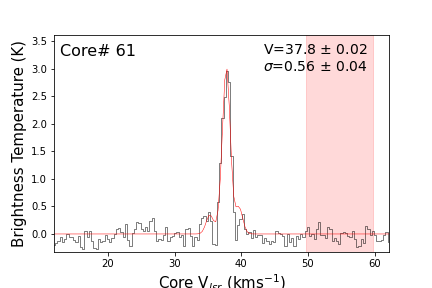}
\includegraphics[width=0.24\textwidth]{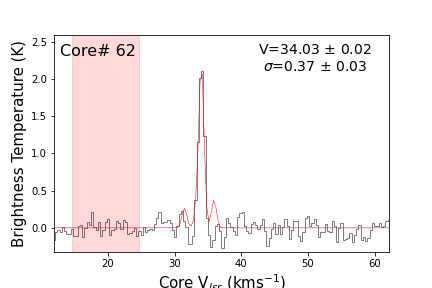}
\includegraphics[width=0.24\textwidth]{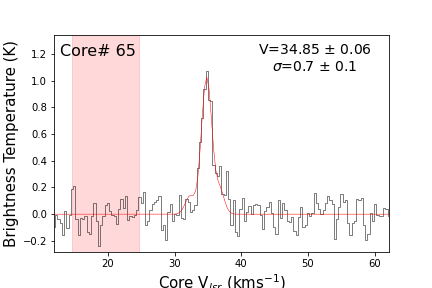}

\caption{Single-type spectra from the background subtracted DCN emission extracted towards the cores in the evolved protocluster G012.80. These spectra are defined as a Single component and used in the analysis. See \cref{tabappendix:coretables_g012} for the line fit parameters for each core.}
\end{figure*}
