# Supplementary material for: ALMA-IMF. VII. First release of the full spectral line cubes: Core kinematics traced by DCN J=(3-2)
Source: arXiv:2306.14710 source file (2023-06-26)
Supplement: Supplementary file 25 [file spw-details-B6.tex]

\begin{table*}[htbp!]
\centering
%\small
%    \setlength{\tabcolsep}{2pt}
%\begin{threeparttable}[c]
\caption{Minimum and maximum frequency ranges [GHz] for the Spectral window setups for B3 spws (0-3).}
%(using global measurements)}
%\label{tab:spwsfreq_1}
\label{tab:spwsfreq}

\begin{tabular}{@{\extracolsep{6pt}}lcccccccc@{}}
 %\begin{tabular}{lrlcrlrlrlrlr}
\hline \noalign {\smallskip}
Protocluster  & \multicolumn{2}{c}{spw0} & \multicolumn{2}{c}{spw1} & \multicolumn{2}{c}{spw2}& \multicolumn{2}{c}{spw3} \\ 
\cline{2-3}\cline{4-5}\cline{6-7}\cline{8-9}
 %\cpartlineleft{1,1em}
%\cline{5-6} \cline{7-8}   
cloud name\tnote{1}  & min & max  & min & max  & min & max  & min & max  \\
\hline \noalign {\smallskip}

G008.67 & 93.103&93.220&91.720&92.656&102.119&103.056&104.519&105.455 \\
G010.62 & 93.116&93.233&91.733&92.669&102.133&103.069&104.533&105.469 \\
G012.80 & 93.103&93.220&91.720&92.657&102.119&103.056&104.519&105.455 \\
G327.29 & 93.129&93.246&91.746&92.682&102.147&103.084&104.547&105.484 \\
G328.25 & 93.128&93.245&91.745&92.682&102.147&103.083&104.547&105.483 \\
G337.92 & 93.127&93.244&91.744&92.681&102.146&103.082&104.546&105.482 \\
G338.93 & 93.134&93.251&91.751&92.688&102.153&103.089&104.554&105.490 \\
G333.60 & 93.130&93.247&91.746&92.683&102.148&103.085&104.548&105.485 \\
G351.77 & 93.116&93.233&91.733&92.669&102.133&103.069&104.533&105.469 \\
G353.41 & 93.120&93.237&91.737&92.674&102.138&103.074&104.538&105.474 \\
W43-MM1 & 93.085&93.202&91.702&92.639&102.099&103.035&104.498&105.434 \\
W43-MM2 & 93.085&93.202&91.702&92.638&102.099&103.035&104.498&105.435 \\
W43-MM3 & 93.085&93.202&91.702&92.639&102.099&103.035&104.498&105.434 \\
W51-E & 93.098&93.215&91.715&92.651&102.113&103.049&104.513&105.449 \\
W51-IRS2 & 93.098&93.215&91.715&92.651&102.113&103.050&104.513&105.449 \\

\hline \noalign {\smallskip}
\end{tabular}
%\begin{tablenotes}

%
%\end{tablenotes}
%\end{threeparttable}
\end{table*}
%\pagestyle{empty}
%\begin{landscape}
\begin{table*}[htbp!]
\ContinuedFloat
\centering
%\small
%    \setlength{\tabcolsep}{2pt}
%\begin{threeparttable}[c]
\caption{Continued: minimum and maximum frequency ranges [GHz] for the Spectral window setups for for B6 spws (0-3).}
%\label{tab:spwsfreq_2}
%(using global measurements)}
\begin{tabular}{@{\extracolsep{6pt}}lcccccccc@{}}
 %\begin{tabular}{lrlcrlrlrlrlr}
\hline \noalign {\smallskip}
Protocluster  & \multicolumn{2}{c}{spw0} & \multicolumn{2}{c}{spw1} & \multicolumn{2}{c}{spw2}& \multicolumn{2}{c}{spw3} \\ 
\cline{2-3}\cline{4-5}\cline{6-7}\cline{8-9}
 %\cpartlineleft{1,1em}
%\cline{5-6} \cline{7-8}   
cloud name\tnote{1}  & min & max  & min & max  & min & max  & min & max  \\
\hline \noalign {\smallskip}
G008.67 & 216.056&216.290&217.006&217.240&219.859&219.976&218.086&218.320 \\
G010.62 & 216.084&216.318&217.034&217.268&219.888&220.005&218.114&218.348 \\
G012.80 & 216.056&216.290&217.006&217.240&219.860&219.976&218.086&218.320 \\
G327.29 & 216.115&216.350&217.066&217.299&219.920&220.036&218.146&218.380 \\
G328.25 & 216.114&216.348&217.064&217.298&219.918&220.035&218.144&218.378 \\
G337.92 & 216.112&216.346&217.062&217.296&219.916&220.033&218.142&218.376 \\
G338.93 & 216.128&216.362&217.078&217.312&219.932&220.049&218.158&218.392 \\
G333.60 & 216.117&216.351&217.067&217.301&219.921&220.038&218.147&218.381 \\
G351.77 & 216.085&216.319&217.035&217.269&219.889&220.006&218.115&218.349 \\
G353.41 & 216.095&216.329&217.045&217.279&219.899&220.016&218.125&218.360 \\
W43-MM1 & 216.014&216.249&216.964&217.198&219.817&219.934&218.044&218.278 \\
W43-MM2 & 216.013&216.247&216.963&217.197&219.816&219.932&218.042&218.276 \\
W43-MM3 & 216.013&216.247&216.963&217.197&219.816&219.932&218.042&218.277 \\
W51-E & 216.043&216.277&216.993&217.227&219.846&219.963&218.073&218.307 \\
W51-IRS2 & 216.043&216.277&216.993&217.227&219.846&219.963&218.073&218.307 \\
\hline \noalign {\smallskip}
\end{tabular}
%\begin{tablenotes}

%\end{tablenotes}
%\end{threeparttable}
\end{table*}

\begin{table*}[htbp!]
\ContinuedFloat
\centering
\caption{Continued: minimum and maximum frequency ranges [GHz] for the Spectral window setups for B6 spws (4-7).}
%\label{tab:spwsfreq_3}
\begin{tabular}{@{\extracolsep{6pt}}lcccccccc@{}}
\hline \noalign {\smallskip}
Protocluster  & \multicolumn{2}{c}{spw4} & \multicolumn{2}{c}{spw5} & \multicolumn{2}{c}{spw6}& \multicolumn{2}{c}{spw7} \\ 
\cline{2-3}\cline{4-5}\cline{6-7}\cline{8-9}
  
cloud name\tnote{1}  & min & max  & min & max  & min & max  & min & max  \\
\hline \noalign {\smallskip}
G008.67 & 219.474&219.591&230.268&230.735&231.017&231.485&231.480&233.353 \\
G010.62 & 219.503&219.620&230.298&230.765&231.047&231.516&231.508&233.381 \\
G012.80 & 219.474&219.591&230.269&230.735&231.017&231.486&231.480&233.353 \\
G327.29 & 219.534&219.651&230.331&230.798&231.081&231.549&231.541&233.414 \\
G328.25 & 219.533&219.650&230.330&230.797&231.079&231.547&231.540&233.413 \\
G337.92 & 219.531&219.648&230.328&230.794&231.077&231.545&231.538&233.361 \\
G338.93 & 219.547&219.664&230.345&230.811&231.094&231.562&231.554&233.426 \\
G333.60 & 219.536&219.653&230.333&230.800&231.082&231.550&231.543&233.415 \\
G351.77 & 219.504&219.621&230.299&230.766&231.048&231.517&231.510&233.383 \\
G353.41 & 219.514&219.631&230.310&230.777&231.059&231.527&231.521&233.393 \\
W43-MM1 & 219.432&219.549&230.224&230.690&230.973&231.441&232.490&234.362 \\
W43-MM2 & 219.431&219.548&230.222&230.689&230.971&231.439&231.436&233.308 \\
W43-MM3 & 219.431&219.547&230.222&230.688&230.971&231.439&231.435&233.308 \\
W51-E & 219.461&219.578&230.255&230.721&231.004&231.472&231.467&233.339 \\
W51-IRS2 & 219.461&219.578&230.255&230.721&231.003&231.472&231.467&233.339 \\
\hline \noalign {\smallskip}
\end{tabular}
\end{table*}
